# Supplementary material for: Equilibration of Quantum hall edges in symmetry broken bilayer graphene
Source: arXiv:1807.07321 source file (2018-07-19)
Supplement: Supplementary file 1 [file SI.pdf]

# Supplementary Material: Equilibration of Quantum hall edges in symmetry broken bilayer graphene

Chandan Kumar, Saurabh Kumar Srivastav, and Anindya Das*
*Department of Physics, Indian Institute of Science, Bangalore 560 012, India*

## I. TWO PROBE CONDUCTANCE AT 10 T

Fig. 1 shows the color plot of two probe conductance at 10 T magnetic field as a function of $V_{BG}$ and $V_{TG}$. The field of 10 T is strong enough to lift the spin, valley and the orbital degeneracy of the zero energy Landau level. This leads to the observation of QH plateaus at integer multiple of $e^2/h$. The horizontal strips represents the back gate filling factor ($\nu_{BG}$) while the diagonal line shows the top gate filling factor ($\nu_{TG}$). Two lines of higher conductance are also observed connecting the unipolar and bipolar region.

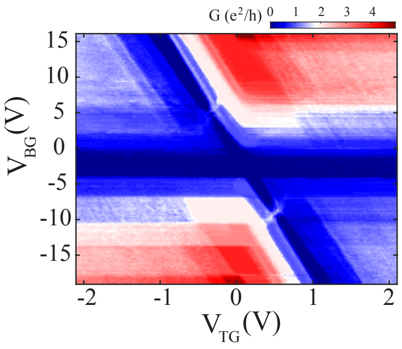


FIG. 1. 2D color map of conductance as a function of $V_{BG}$ and $V_{BG}$ at 10 T magnetic field. The horizontal and diagonal strips represents the back gate and top gate filling fraction.

## II. EDGE STATE EQUILIBRATION IN FOUR PROBE GEOMETRY

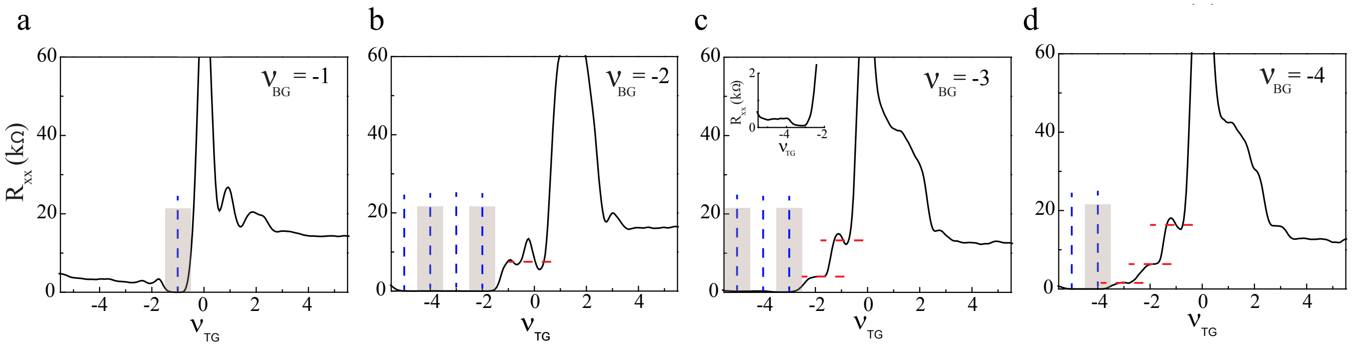


FIG. 2. $R_{xx}$ as a function of $\nu_{TG}$ at different set of $\nu_{BG}$ at 10 T and 40 mK for (a) $\nu_{BG} = -1$ (b) $\nu_{BG} = -2$ (c) $\nu_{BG} = -3$ (d) $\nu_{BG} = -4$. For $\nu_{BG} = -2(\nu_{BG} = -4)$ the resistance is zero from $\nu_{TG} = -2$ to $\nu_{TG} = -5$ ($\nu_{TG} = -4$ to $\nu_{TG} = -5$), suggesting that these edge states do not equilibrate in our device. The dashed red line represent different QH plateaus expected for full equilibration of QH edge states in unipolar regime.

* anindya@iisc.ac.in

Figure 2 shows the four probe resistance as a function of $\nu_{TG}$ for different set of $\nu_{BG}$. As can be seen from Fig.2b, for $\nu_{BG} = -2$, the resistance is zero for $\nu_{TG} = -2$ to $\nu_{TG} = -5$. Implying that these edge states pass through the top gate region without any scattering. Similarly, we find that for $\nu_{BG} = -4$, the resistance is zero for $\nu_{TG} = -4$ to $\nu_{TG} = -5$. This suggest that these edge states do not equilibrate in our device. This is consistent with the two probe measurement presented in the main manuscript.
